# Supplementary material for: On Locally Decodable Codes in Resource Bounded Channels
Source: arXiv:1909.11245 source file (2020-06-05)
Supplement: Supplementary file 1 [file appendix_prom.tex]

\section{\pROM Model} \label{appendix:pROM}
A \pROM algorithm is a probabilistic turing machine having query access to a random oracle. As noted in \cite{STOC:AlwSer15}, the exact model of computation is not too important and any type of algorithms may be used; however, we use turing machines for simplicity. Interactions of the algorithm with the random oracle are made through \emph{rounds} and such interactions are termed as \emph{round based interactions}. Formally, the round based interaction for a stateless oracle $\oracleO$ and oracle turing machine $\oracletmTO$ with oracle access to $\oracleO$ and on input $x$ may be described as follows: During the $i$th round,

\begin{itemize}
    \item $\oracletmTO$ receives  $(\sigma_i, a^{(i)})$ as input. Here $\sigma_i$ is the state of the machine, and $a^{(i)} = (a^{(i)}_1, a^{(i)}_2, \cdots , a^{(i)}_{p_{i-1}})$ are the answers to the batch of queries $q_{i-1}$ of the previous round. For $i = 0, \sigma_i =x$ and $a_i = \{\}$
    \item $\oracletmTO$ may choose to perform arbitrary computation to update contents of its memory and output a new state $\sigma_{i+1}$ along with a new batch of $p_i$ queries $q^{(i)} = (q^{(i)}_1, q^{(i)}_2, \cdots , q^{(i)}_{p_{i}})$ to submit to the random oracle.
    \item The entire batch $q^{(i)}$ is handed to the random oracle. This concludes the round.
\end{itemize}

\noindent $\oracletmTO$ also has an output tape onto which it may append output values at any time. A special character $\bot$ is designated to signal termination, and the round based interaction is said to \emph{terminate} when $\oracletmTO$ writes $\bot$ to the end of the output. If the interaction terminates in $t$ rounds, we call it a $t$-round interaction.  $\abs{\sigma_i}$ denotes the \emph{size} of the state $\sigma_i$, which is the minimum number of bits required to encode any necessary state information.
